# Supplementary material for: Bregman Deviations of Generic Exponential Families
Source: arXiv:2201.07306 source file (2023-07-13)
Supplement: Supplementary file 1 [file technical.tex]

\section{TECHNICAL DETAILS}

$
(n\!+\!c)\cB_\cL \left(\theta,\theta_{n,c}(\theta)			\right)\geq \log(1/\delta)+\gamma_{n,c}(\theta)
$

For Bernoulli distributions, it holds that
\begin{align}
\gamma_{n,c}(\theta)=& (S_n + c\mu)\log \mu_{n,c}(\mu) + \left(n-S_n+c(1-\mu)\right)\log (1-\mu_{n,c}(\mu))-c\mu \log \mu - c(1-\mu)\log (1-\mu)\nonumber\\&+
\log \frac{\Gamma(c\mu)\Gamma(c(1-\mu))}{\Gamma(S_n+c\mu)\Gamma(n-S_n+c(1-\mu))} + \log \frac{\Gamma(n+c)}{\Gamma(c)}~. 
\end{align}
In particular, 
\beqan
\gamma_{n,c}(\theta)&=& (n+c)\cB_\cL(\theta,\theta_{n,c}(\theta)) + S_n \log(\mu) + (n-S_n)\log(1-\mu)\\
&&+\log \frac{\Gamma(c\mu)\Gamma(c(1-\mu))}{\Gamma(S_n+c\mu)\Gamma(n-S_n+c(1-\mu))} + \log \frac{\Gamma(n+c)}{\Gamma(c)}~. 
\eeqan

%
%\begin{align}
%\gamma_{n,c}(\theta)=& (n+c) \mu_{n,c}(\mu)\log(\frac{\mu_{n,c}(\mu)}{1-\mu_{n,c}(\mu)}) + (n+c)\log (1-\mu_{n,c}(\mu)) + c\mu \log(\frac{1-\mu}{\mu}) - c\log (1-\mu)\nonumber\\&+
%\log \frac{\Gamma(c\mu)\Gamma(c(1-\mu))}{\Gamma( (n+c) \mu_{n,c}(\mu) )\Gamma((n+c)(1- \mu_{n,c}(\mu)))} + \log \frac{\Gamma(n+c)}{\Gamma(c)}~. 
%\end{align}
Now using $h(x)=x\log(x)$, and $\tilde \mu = \mu_{n,c}(\mu)$ it comes

\begin{align}
\gamma_{n,c}(\theta)=& (n+c)\big[h(\tilde \mu)+ h(1-\tilde \mu)\big] -c \big[h(\mu)+ h(1-\mu)\big]\nonumber\\&+
\log \frac{\Gamma(c\mu)\Gamma(c(1-\mu))}{\Gamma( (n+c) \tilde \mu )\Gamma((n+c)(1- \tilde \mu))} + \log \frac{\Gamma(n+c)}{\Gamma(c)}~. 
\end{align}

By Stirling Formula, it comes
$$\log (\Gamma(z_1)/\Gamma(z_2)) =  (z_1-1/2)\log(z_1)-z_1 -(z_2-1/2)\log(z_2)+z_2   + \log(1+O(z_1^{-1}))- \log(1+O(z_2^{-1}))$$
\beqan
\log \frac{\Gamma(c\mu)\Gamma(c(1-\mu))}{\Gamma( (n+c) \tilde \mu )\Gamma((n+c)(1- \tilde \mu))} = 
\eeqan
